# Supplementary material for: Heterogeneous Peer Effects in the Linear Threshold Model
Source: arXiv:2201.11242 source file (2022-01-27)
Supplement: Supplementary file 4 [file synthetic_mse_figures_appendix.tex]

\begin{figure*}[!ht]
	\centering
    \begin{subfigure}{\legendsize}
        \includegraphics[width=\textwidth]{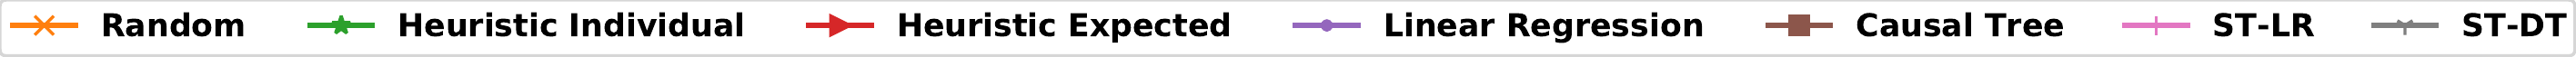}    
    \end{subfigure}

	\begin{subfigure}[b]{\subfiguresize}
		\includegraphics[width=\textwidth]{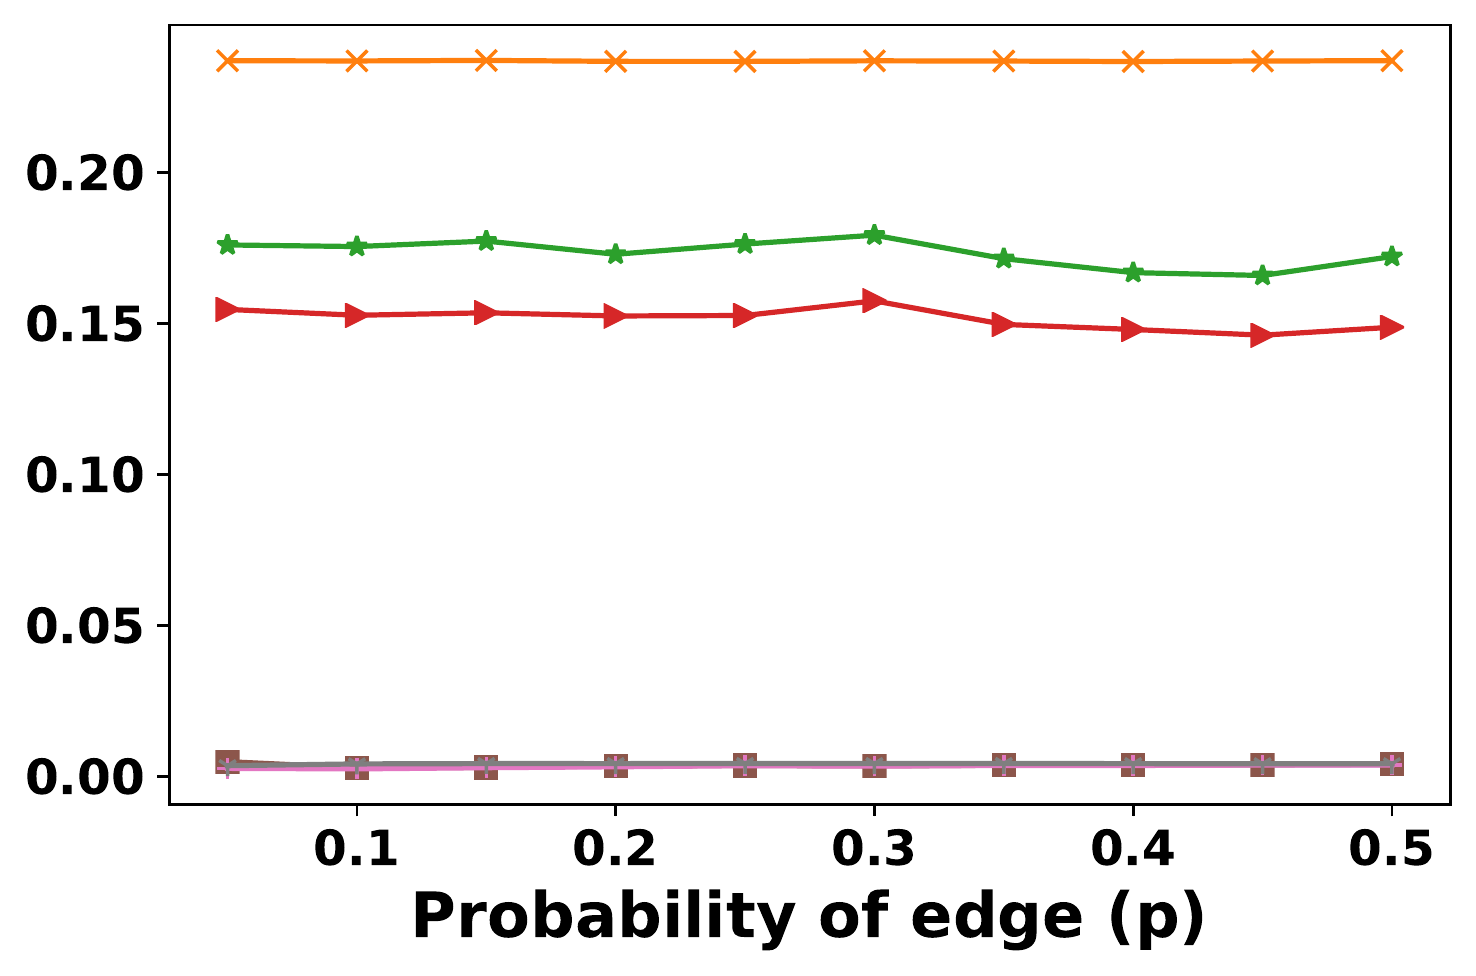}
		\caption{Erdos-Renyi}\label{fig:linear-erdos}
	\end{subfigure}
	\begin{subfigure}[b]{\subfiguresize}
		\includegraphics[width=\textwidth]{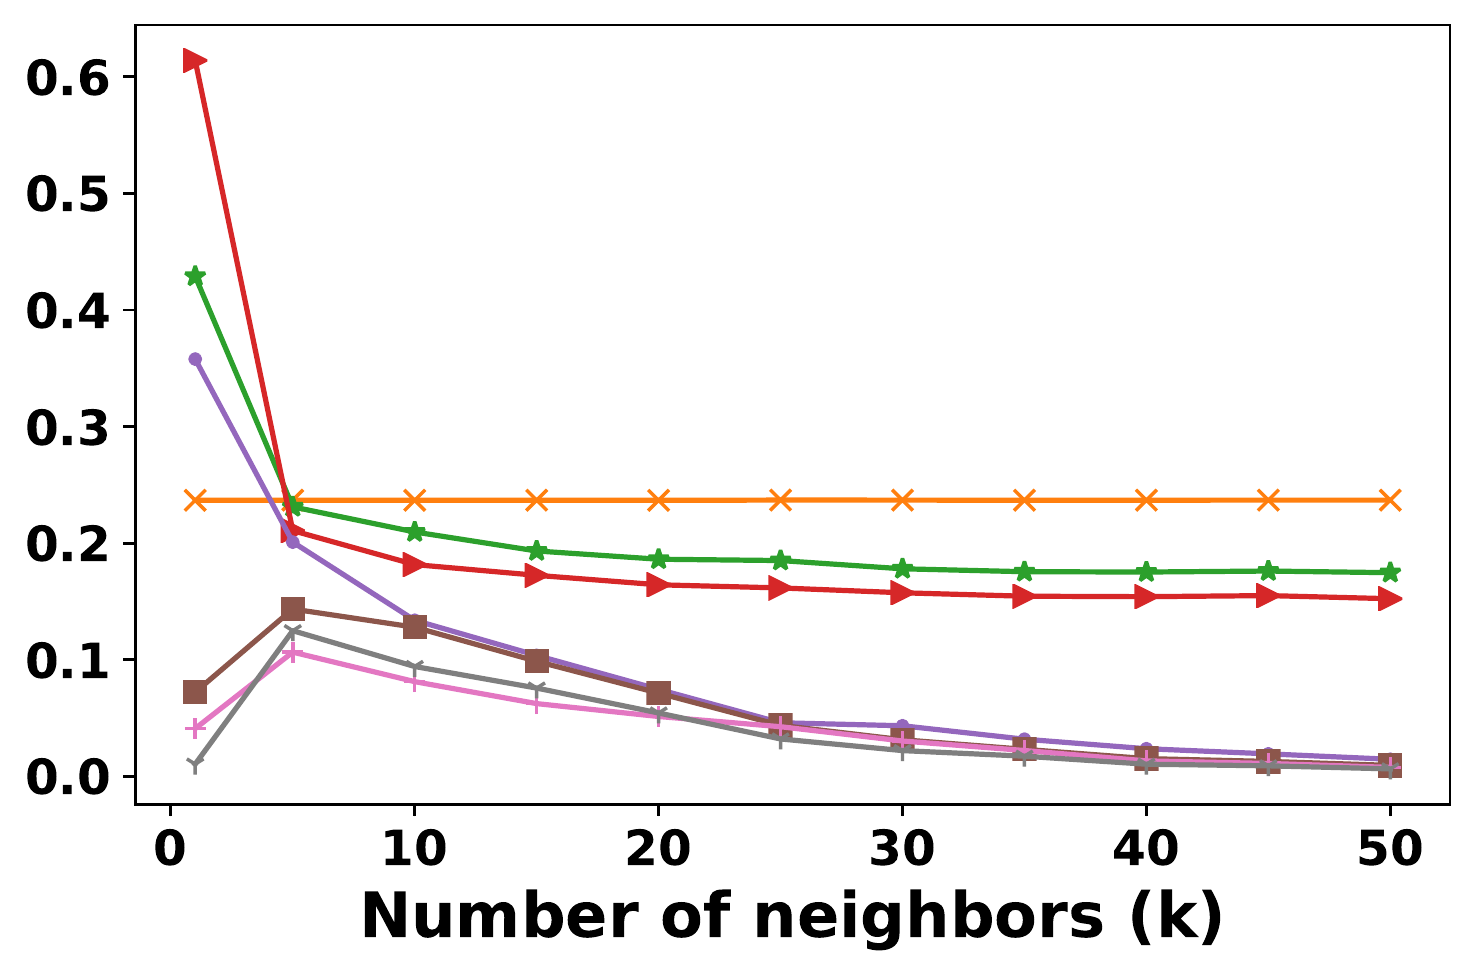}
		\caption{Pref. attachment}\label{fig:linear-pref}
	\end{subfigure}
	\begin{subfigure}[b]{\subfiguresize}
		\includegraphics[width=\textwidth]{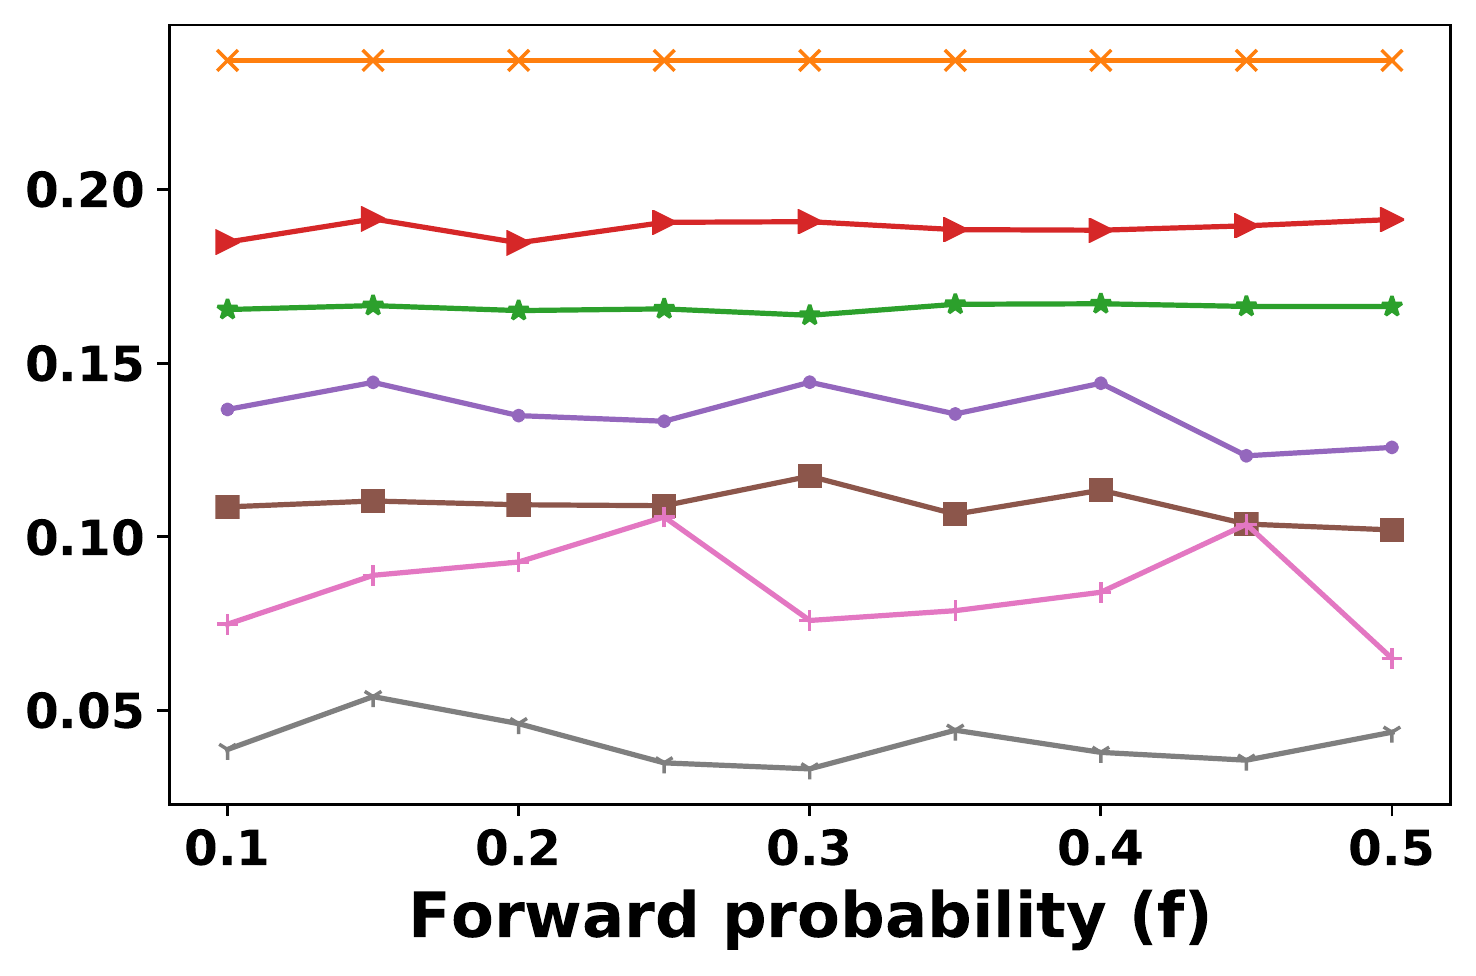}
		\caption{Forest fire}\label{fig:linear-forest}
	\end{subfigure}
	\begin{subfigure}[b]{\subfiguresize}
		\includegraphics[width=\textwidth]{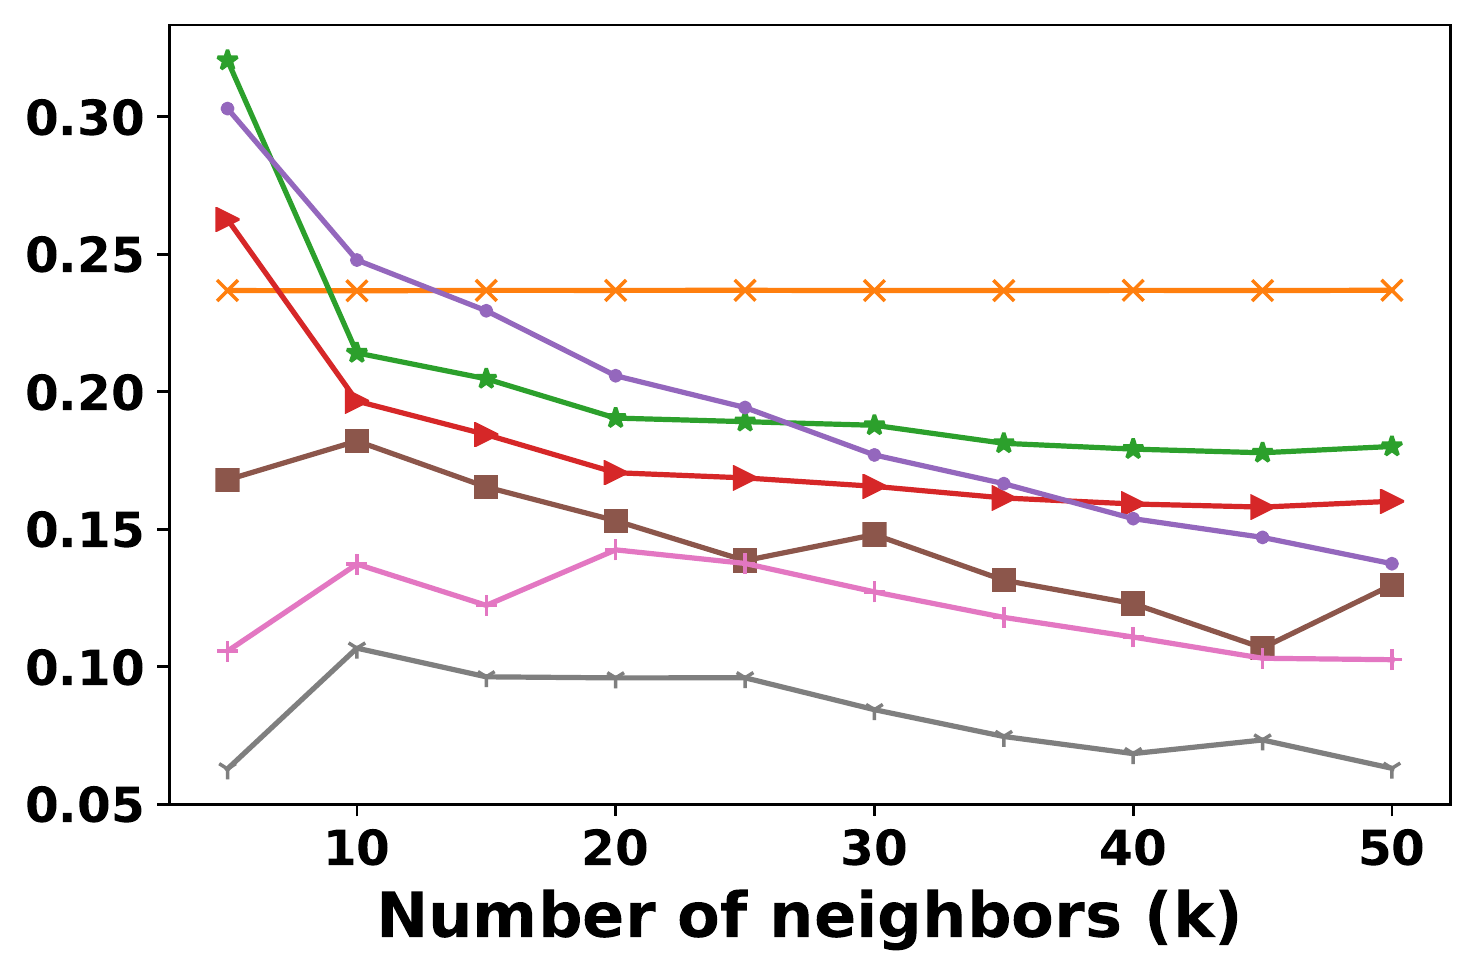}
		\caption{Watts-Strogatz}\label{fig:linear-watts}
	\end{subfigure}

	\begin{subfigure}[b]{\subfiguresize}
		\includegraphics[width=\textwidth]{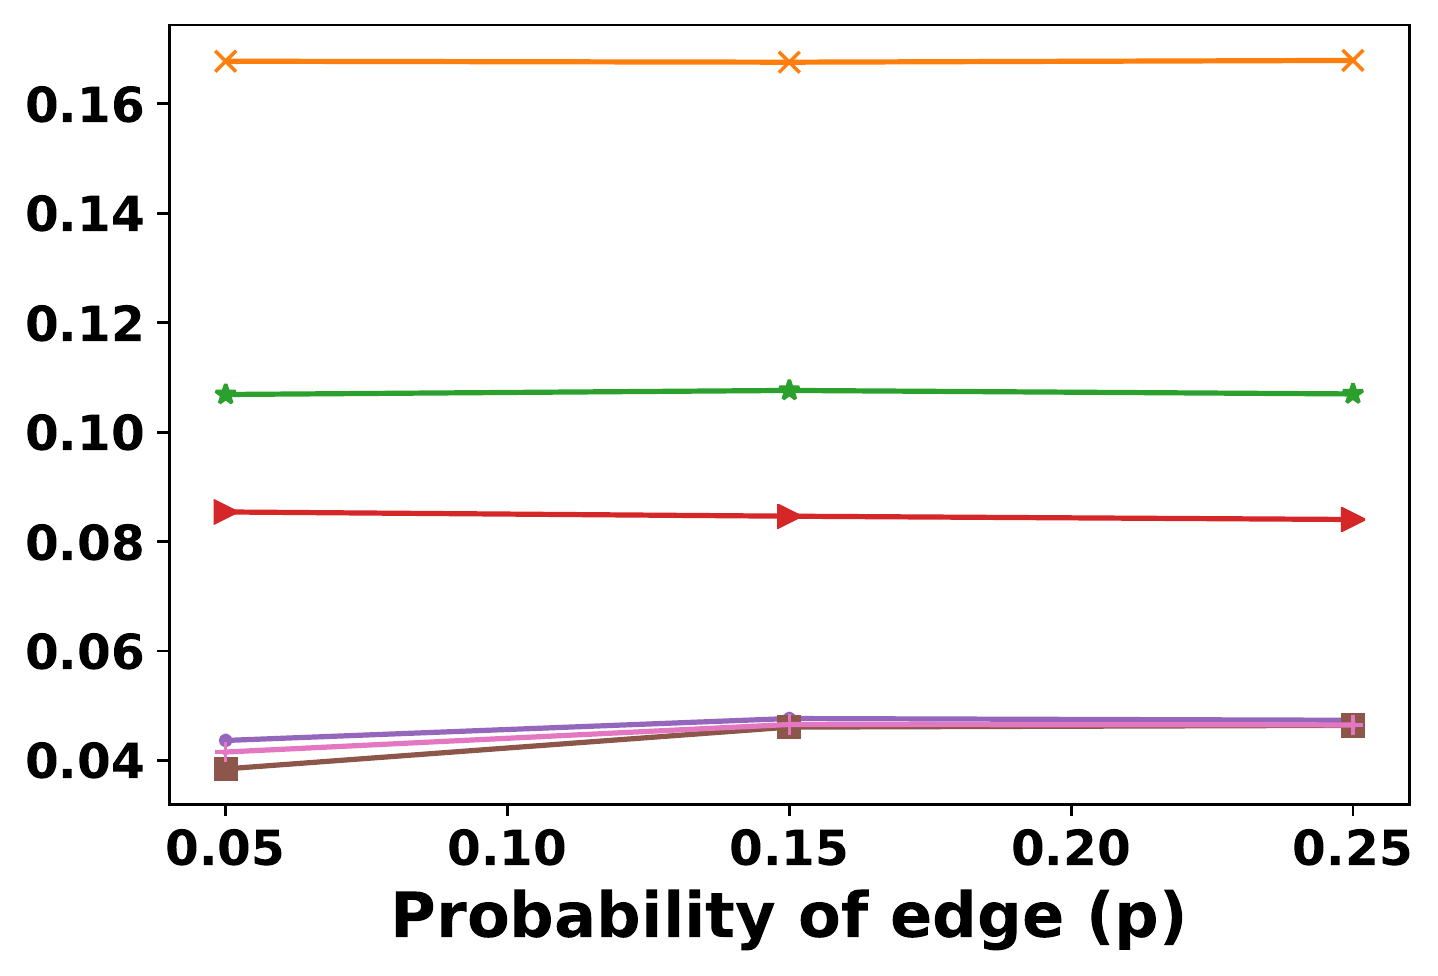}
		\caption{Erdos-Renyi}\label{fig:quad-erdos}
	\end{subfigure}
	\begin{subfigure}[b]{\subfiguresize}
		\includegraphics[width=\textwidth]{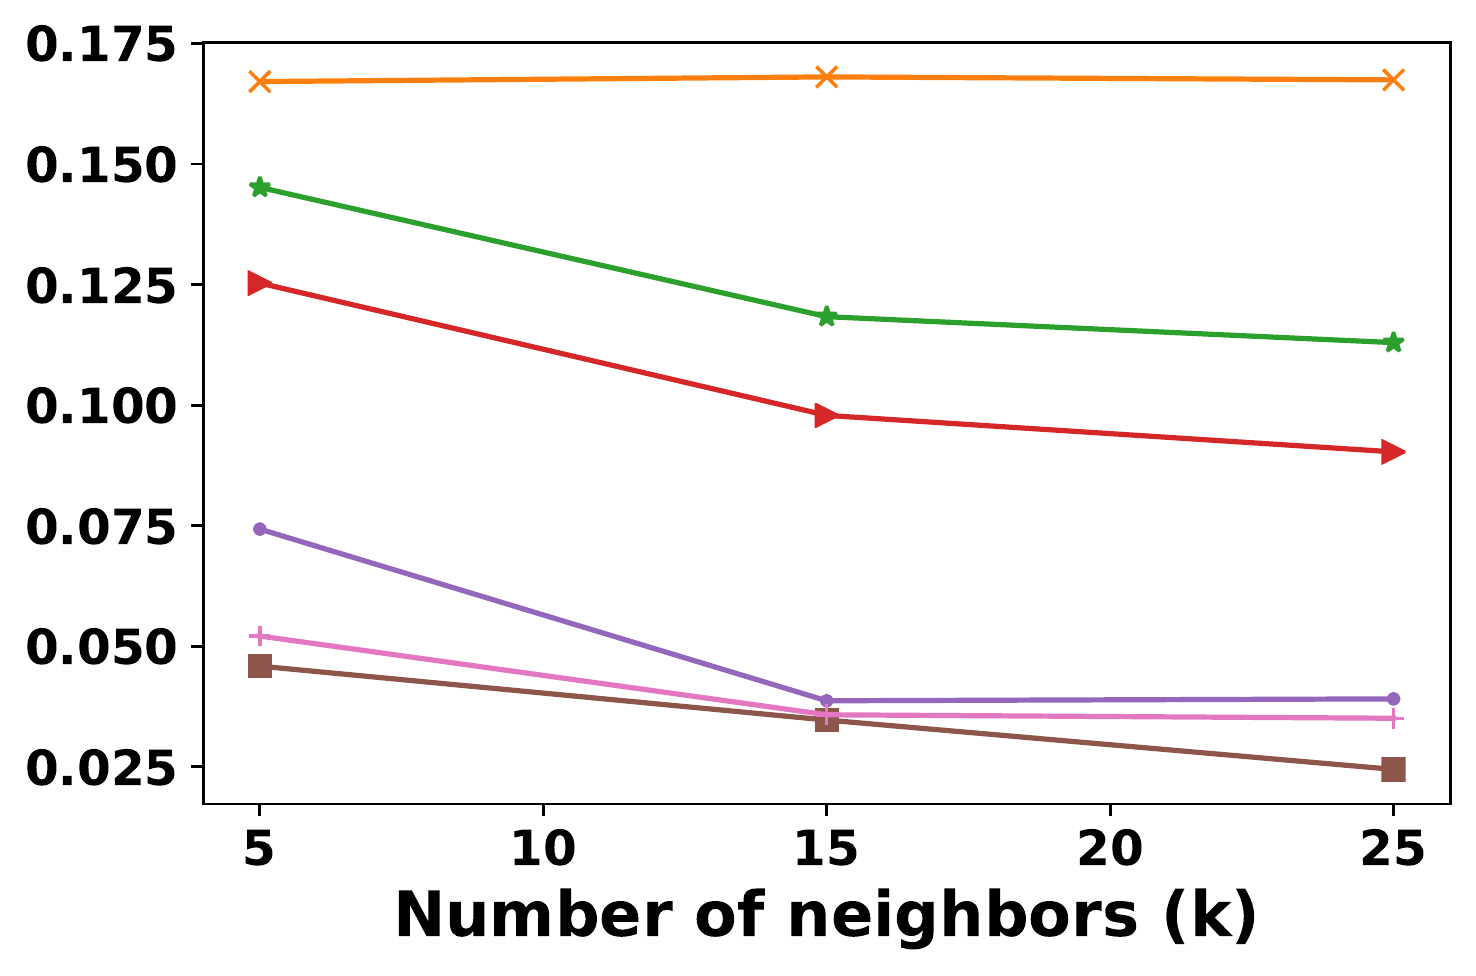}
		\caption{Pref. attachment}\label{fig:quad-pref}
	\end{subfigure}
	\begin{subfigure}[b]{\subfiguresize}
		\includegraphics[width=\textwidth]{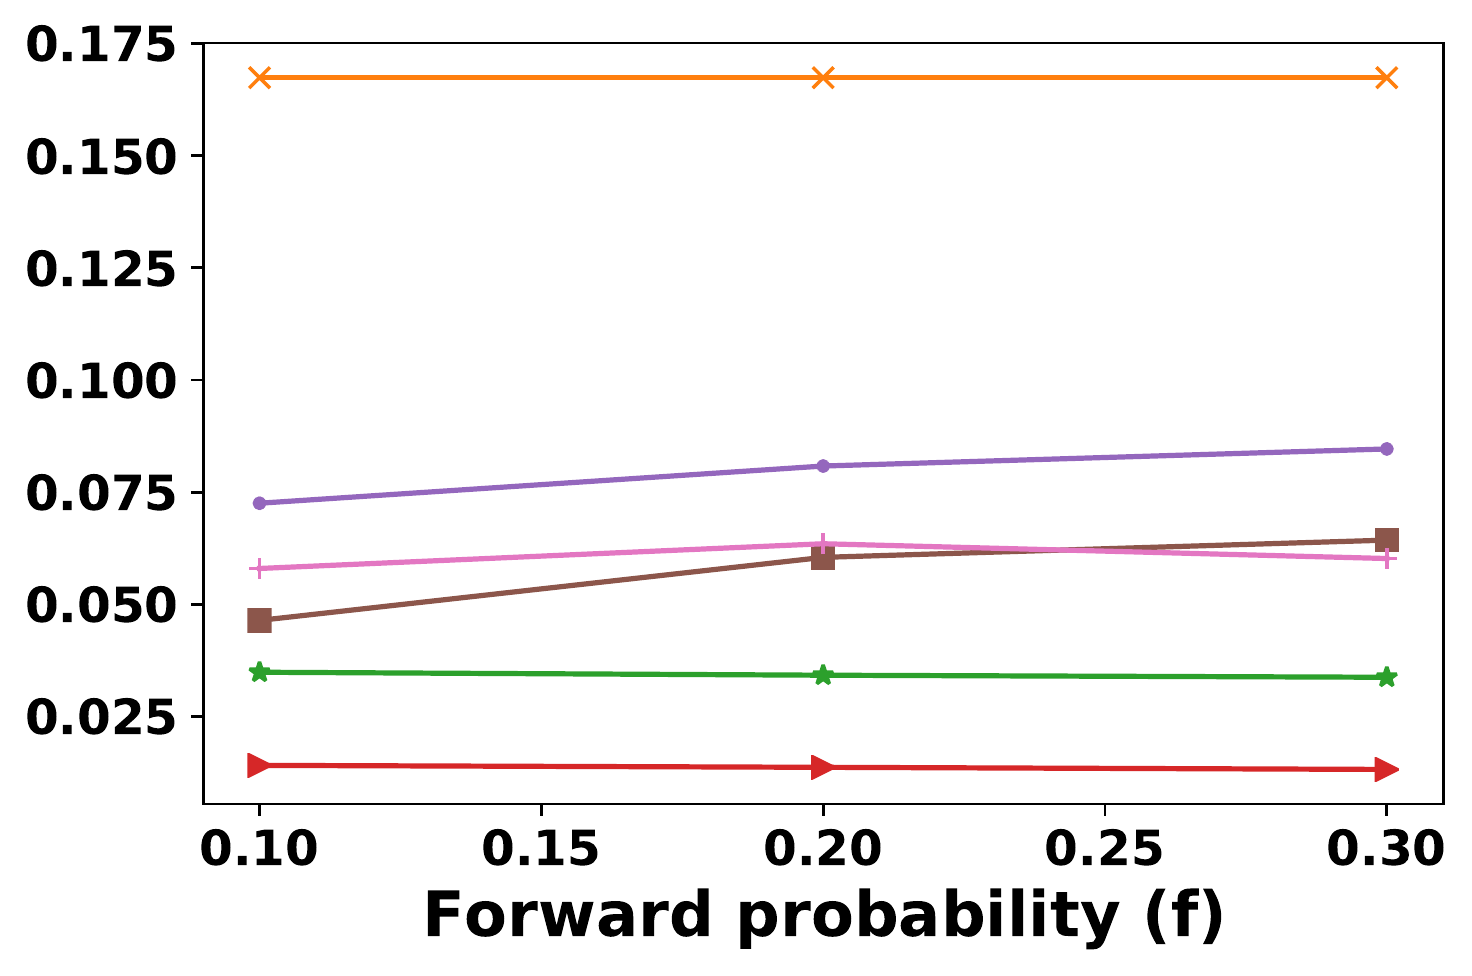}
		\caption{Forest fire}\label{fig:quad-forest}
	\end{subfigure}
	\begin{subfigure}[b]{\subfiguresize}
		\includegraphics[width=\textwidth]{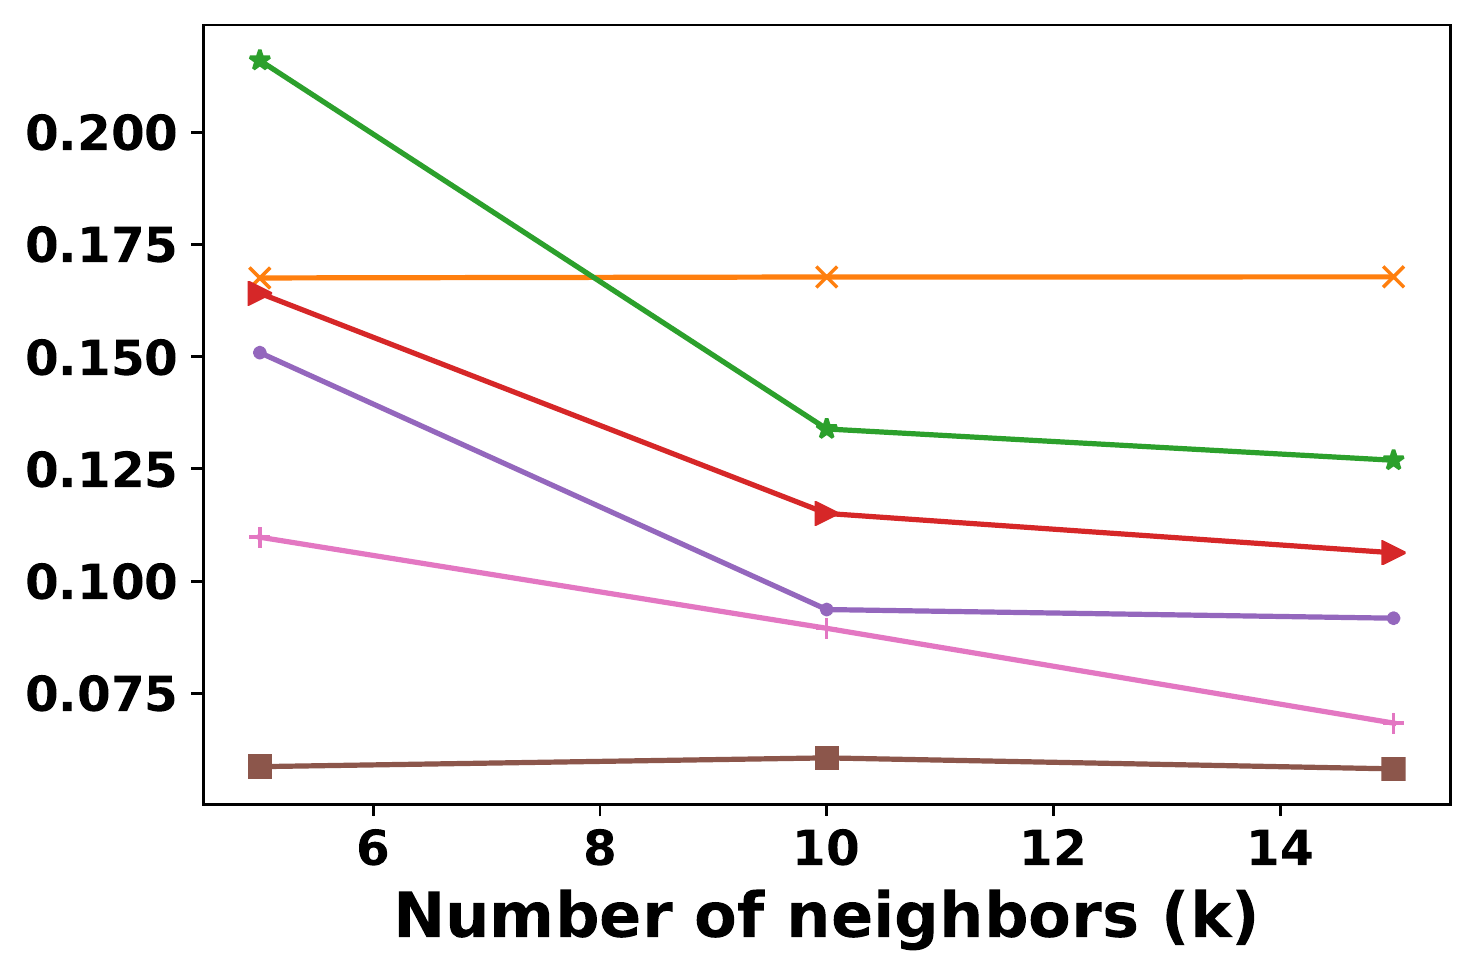}
		\caption{Watts-Strogatz}\label{fig:quad-watts}
	\end{subfigure}
	\caption{\kdd{MSE of threshold prediction for the \emph{Linear} (top row) and \emph{Quadrant} (bottom row) setups over different parameters.}}\label{fig:synthetic_mse_appendix}
\end{figure*}
